# Supplementary material for: Contamination Report for Multilingual Benchmarks
Source: arXiv:2410.16186 source file (2024-10-21)
Supplement: Supplementary file 1 [file appendix.tex]

\section{Appendix}
\subsection{Previous Results}

\begin{table}[h]
\small 
\centering
\begin{tabular}{@{}l|ccc@{}}
\toprule
 & \textsc{Gemma-7B-it} & \textsc{Llama-2-7B-it} & \textsc{Mistral-7B-v0.1-it} \\ \midrule
\textsc{Paws-X}     & \xmark & \xmark & \xmark \\
\textsc{XCopa}      & \xmark & \xmark & \xmark \\
\textsc{Xnli}       & \cmark & \cmark & \cmark \\
\textsc{XQuad}     & \cmark & \xmark & \xmark \\
\textsc{XStoryCloze} & \cmark & \cmark & \cmark \\ \bottomrule
\end{tabular}
 \vspace{2mm}
\caption{Previous contamination results from \citet{ahuja-etal-2024-megaverse}. We use this table for cross-comparison.}
\label{tab:previous_results}
\end{table}
